# Supplementary material for: Label merge-and-split: A graph-colouring approach for memory-efficient brain parcellation
Source: arXiv:2404.10572 source file (2024-08-01)

# Label merge-and-split: A graph-colouring approach for memory-efficient brain parcellation

## Supplementary Materials

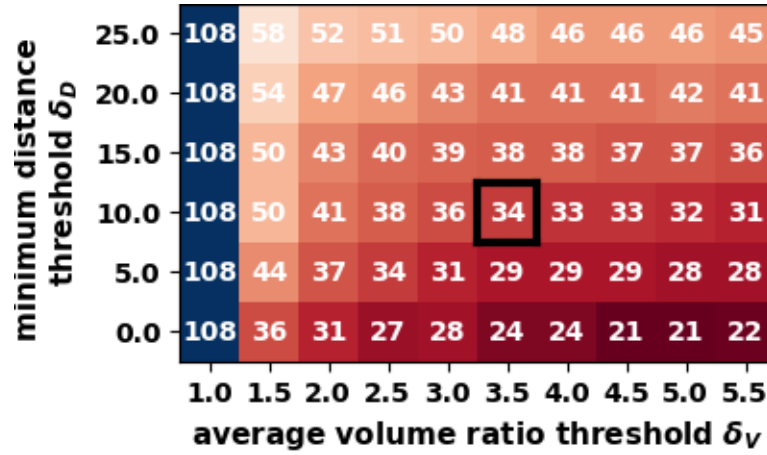

**Figure A:** Number of effective labels resulting from the graph coloring algorithm depending on the minimum distance and average volume ratio thresholds for the AOMIC dataset. The chosen values are highlighted with a black box.

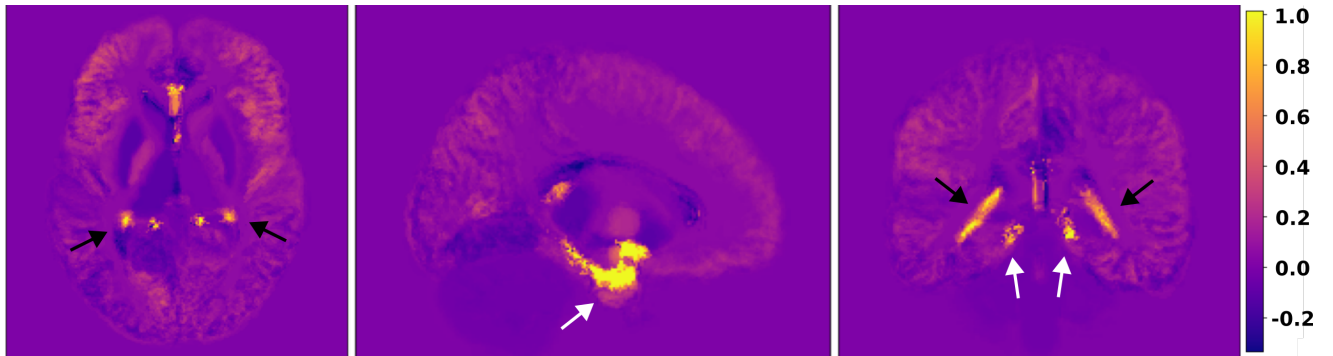

**Figure B:** Earlier results without volume ratio threshold showed reduced segmentation accuracy of small structures due to large class imbalance within merged label groups. Regions where the merged model performed worse/better are yellow/blue. Small structures (chorioid plexus: black arrows; entorhinal cortex: white arrows) that were merged with much larger structures were segmented less accurately. The average volume ratio threshold was introduced to mitigate class imbalance within merged label groups.

**Table A:** Additional metrics for all experiments: relative volume error (RVE) and Hausdorff distance to complement the Dice Similarity Coefficient of Table 1 of the main paper. Bold numbers indicate the better value when comparing merged and original model.

|                         | RVE [%]          |                    |                    | Hausdorff [mm]     |                    |                    |
|-------------------------|------------------|--------------------|--------------------|--------------------|--------------------|--------------------|
|                         | test set         |                    |                    | test set           |                    |                    |
|                         | AOMIC            | IXI                | Mindboggle42       | AOMIC              | IXI                | Mindboggle42       |
| AOMIC <sub>orig</sub>   | <b>5.7 (7.9)</b> | <b>10.1 (10.3)</b> | <b>16.0 (15.1)</b> | <b>7.89 (6.07)</b> | <b>8.46 (6.31)</b> | <b>9.19 (6.92)</b> |
| AOMIC <sub>merged</sub> | 5.8 (7.9)        | 10.6 (11.2)        | 16.4 (15.6)        | 7.99 (6.22)        | 8.78 (6.76)        | 9.32 (7.74)        |
| IXI <sub>orig</sub>     | 8.2 (8.9)        | 5.4 (7.5)          | 16.5 (15.7)        | <b>7.94 (5.85)</b> | <b>7.92 (5.77)</b> | <b>8.92 (6.84)</b> |
| IXI <sub>merged</sub>   | <b>7.4 (8.5)</b> | <b>5.2 (7.1)</b>   | <b>16.0 (15.4)</b> | 8.07 (6.25)        | 8.1 (5.97)         | 8.94 (7.02)        |

# Label merge-and-split: A graph-colouring approach for memory-efficient brain parcellation

## Supplementary Materials

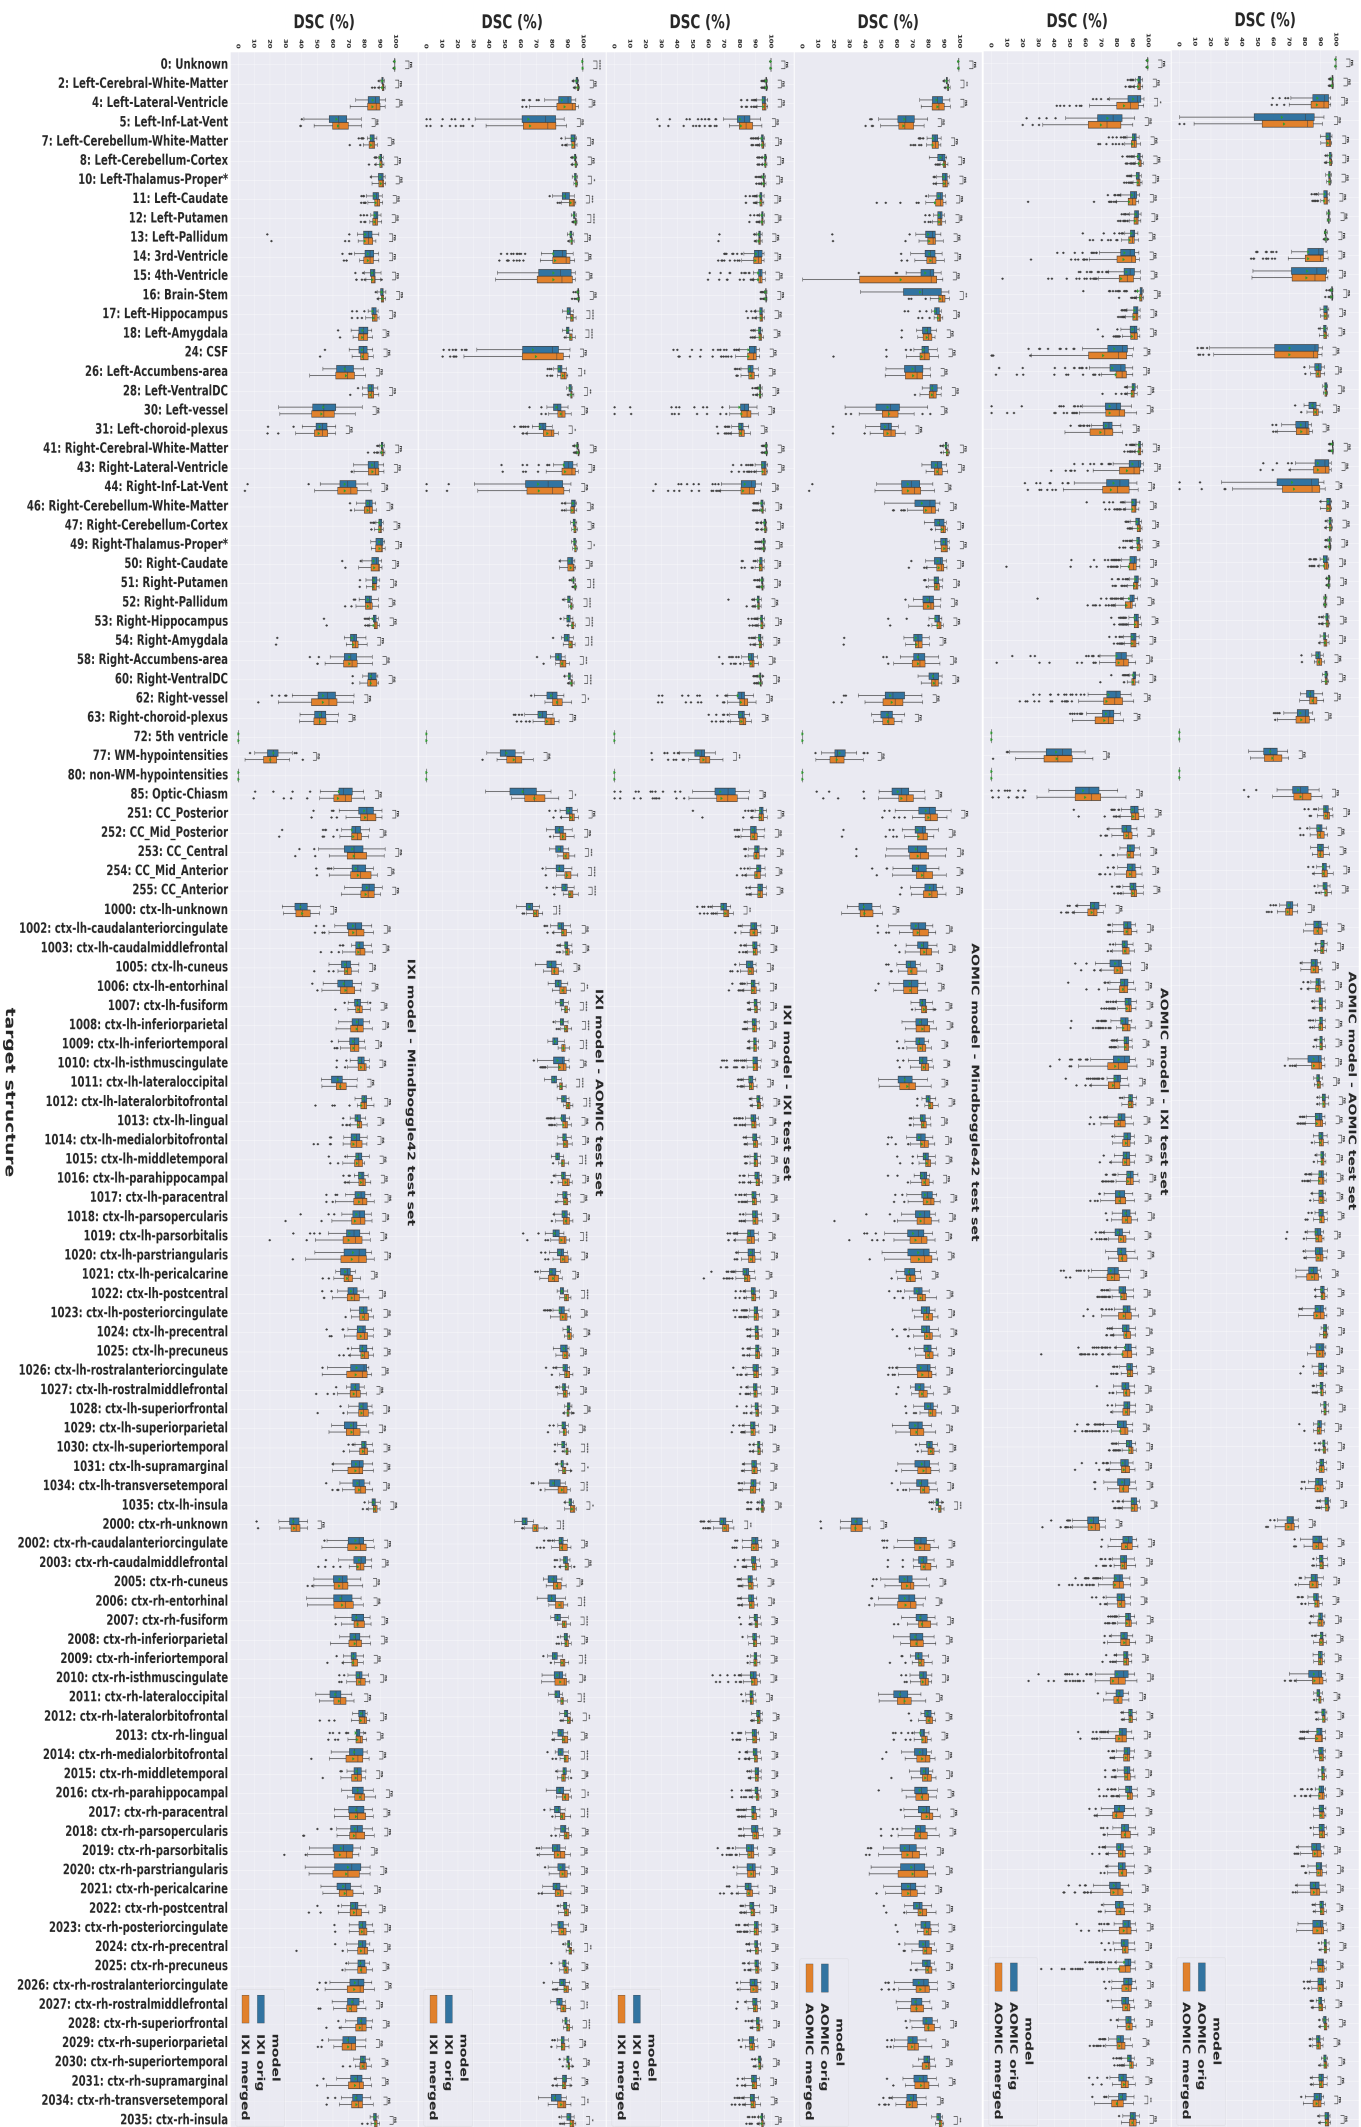

Supplement: Supplementary file 1 [file supplementary_materials.pdf]
